# Supplementary material for: IsoVRBench: Video Reward Modeling Without Human Feedback
Source: arXiv:2610.17234 source file (2026-10-12)
Supplement: Supplementary file 1 [file appendix.tex]

\appendix
\section{Appendix}
